# Supplementary material for: Perturbation Theory Treatment of Spin-Orbit Coupling. III: Coupled Perturbed Method for Solids
Source: arXiv:2302.06143 source file (2023-02-13)
Supplement: Supplementary file 1 [file Part_4_SI.pdf]

# Perturbation Theory Treatment of Spin-Orbit Coupling. III: Coupled Perturbed Method for Solids

Jacques K. Desmarais,* Alberto Boccuni, and Alessandro Erba†
*Dipartimento di Chimica, Università di Torino, via Giuria 5, 10125 Torino, Italy*

Jean-Pierre Flament
*Université de Lille, CNRS, UMR 8523 — PhLAM — Physique des Lasers, Atomes et Molécules, 59000 Lille, France*

Bernard Kirtman
*Department of Chemistry and Biochemistry, University of California, Santa Barbara, California 93106, USA*

*Electronic address: jacqueskontak.desmarais@unito.it
†Electronic address: alessandro.erba@unito.it

## I. DERIVATION OF TOTAL ENERGY FORMULAS

## II. ENERGY FORMULAS

Following Eq. (57) and Eqs. (A1a)-(A1d) of Paper 2 [1], we write the total energy of the periodic system in orders of perturbation theory as:

$$E = E^{(0)} + \lambda E^{(1)} + \lambda^2 E^{(2)} + \lambda^3 E^{(3)} + \dots \tag{S1a}$$

$$E^{(0)} = \frac{1}{2}\sum_{\sigma}\sum_{\mathbf{g}} \Re\mathrm{Tr}\left[\left(\mathbf{v}(\mathbf{g}) + \mathbf{u}_{AR}(\mathbf{g}) + \mathbf{H}^{\sigma\sigma(0)}(\mathbf{g})\right)\mathbf{P}^{\sigma\sigma(0)}(\mathbf{g})\right] \tag{S1b}$$

$$\begin{aligned} E^{(1)} &= \frac{1}{2}\sum_{\sigma}\sum_{\mathbf{g}} \Re\mathrm{Tr}\left[\left(\mathbf{v}(\mathbf{g}) + \mathbf{u}_{AR}(\mathbf{g}) + \mathbf{H}^{\sigma\sigma(0)}(\mathbf{g})\right)\mathbf{P}^{\sigma\sigma(1)}(\mathbf{g})\right] \\ &+ \frac{1}{2}\sum_{\sigma}\sum_{\mathbf{g}} \Re\mathrm{Tr}\left[\left(\mathbf{V}^{\sigma\sigma(1)}(\mathbf{g}) - a\mathbf{K}^{\sigma\sigma(1)}(\mathbf{g})\right)\mathbf{P}^{\sigma\sigma(0)}(\mathbf{g})\right] \\ &+ \sum_{\sigma}\sum_{\mathbf{g}} \Re\mathrm{Tr}\left[\mathbf{u}_{SO}^{\sigma\sigma}(\mathbf{g})\mathbf{P}^{\sigma\sigma(0)}(\mathbf{g})\right] \end{aligned} \tag{S1c}$$

$$\begin{aligned} E^{(2)} &= \frac{1}{2}\sum_{\sigma}\sum_{\mathbf{g}} \Re\mathrm{Tr}\left[\left(\mathbf{v}(\mathbf{g}) + \mathbf{u}_{AR}(\mathbf{g}) + \mathbf{F}^{\sigma\sigma(0)}(\mathbf{g})\right)\mathbf{P}^{\sigma\sigma(2)}(\mathbf{g})\right] \\ &+ \frac{1}{2}\sum_{\sigma\sigma'}\sum_{\mathbf{g}} \Re\mathrm{Tr}\left[\left(\mathbf{V}^{\sigma\sigma'(1)}(\mathbf{g}) - a\mathbf{K}^{\sigma\sigma'(1)}(\mathbf{g})\right)\mathbf{P}^{\sigma'\sigma(1)}(\mathbf{g})\right] \\ &+ \frac{1}{2}\sum_{\sigma}\sum_{\mathbf{g}} \Re\mathrm{Tr}\left[\left(\mathbf{C}^{\sigma\sigma(2)}(\mathbf{g}) + \mathbf{V}^{\sigma\sigma(2)}(\mathbf{g}) - a\mathbf{K}^{\sigma\sigma(2)}(\mathbf{g})\right)\mathbf{P}^{\sigma\sigma(0)}(\mathbf{g})\right] \\ &+ \sum_{\sigma\sigma'}\sum_{\mathbf{g}} \Re\mathrm{Tr}\left[\mathbf{u}_{SO}^{\sigma\sigma'}(\mathbf{g})\mathbf{P}^{\sigma'\sigma(1)}(\mathbf{g})\right] \end{aligned} \tag{S1d}$$

$$\begin{aligned} E^{(3)} &= \frac{1}{2}\sum_{\sigma}\sum_{\mathbf{g}} \Re\mathrm{Tr}\left[\left(\mathbf{v}(\mathbf{g}) + \mathbf{u}_{AR}(\mathbf{g}) + \mathbf{H}^{\sigma\sigma(0)}(\mathbf{g})\right)\mathbf{P}^{\sigma\sigma(3)}(\mathbf{g})\right] \\ &+ \frac{1}{2}\sum_{\sigma\sigma'}\sum_{\mathbf{g}} \Re\mathrm{Tr}\left[\left(\mathbf{V}^{\sigma\sigma'(1)}(\mathbf{g}) - a\mathbf{K}^{\sigma\sigma'(1)}(\mathbf{g})\right)\mathbf{P}^{\sigma'\sigma(2)}(\mathbf{g})\right] \\ &+ \frac{1}{2}\sum_{\sigma\sigma'}\sum_{\mathbf{g}} \Re\mathrm{Tr}\left[\left(\mathbf{C}^{\sigma\sigma'(2)}(\mathbf{g}) + \mathbf{V}^{\sigma\sigma'(2)}(\mathbf{g}) - a\mathbf{K}^{\sigma\sigma'(2)}(\mathbf{g})\right)\mathbf{P}^{\sigma'\sigma(1)}(\mathbf{g})\right] \\ &+ \frac{1}{2}\sum_{\sigma}\sum_{\mathbf{g}} \Re\mathrm{Tr}\left[\left(\mathbf{C}^{\sigma\sigma(3)}(\mathbf{g}) + \mathbf{V}^{\sigma\sigma(3)}(\mathbf{g}) - a\mathbf{K}^{\sigma\sigma(3)}(\mathbf{g})\right)\mathbf{P}^{\sigma\sigma(0)}(\mathbf{g})\right] \\ &+ \sum_{\sigma\sigma'}\sum_{\mathbf{g}} \Re\mathrm{Tr}\left[\mathbf{u}_{SO}^{\sigma\sigma'}(\mathbf{g})\mathbf{P}^{\sigma'\sigma(2)}(\mathbf{g})\right] \end{aligned} \tag{S1e}$$

### A. Zeroth-Order Energy

The simplified zeroth-order energy expression can be obtained by substituting Eqs. (37a) and (38) into Eq. (S1b) to find:

$$\begin{aligned} E^{(0)} &= \frac{1}{\Omega}\sum_{\sigma}\sum_{\mathbf{g}} \Re\mathrm{Tr}\left\{ \int' d\mathbf{k} e^{\imath\mathbf{k}\cdot\mathbf{g}} \left(\mathbf{v}(\mathbf{g}) + \mathbf{u}_{AR}(\mathbf{g}) + \mathbf{H}^{\sigma\sigma(0)}(\mathbf{g})\right) \right. \\ &\times \left. \mathbf{C}^{\sigma\sigma(0)}(\mathbf{k})\mathbf{f}_{\sigma}(\mathbf{k})\left[\mathbf{C}^{\sigma\sigma(0)}(\mathbf{k})\right]^{\dagger} \right\} \end{aligned} \tag{S2}$$

Now using:

$$\mathbf{v}(\mathbf{k}) = \sum_{\mathbf{g}} e^{\imath\mathbf{k}\cdot\mathbf{g}}\mathbf{v}(\mathbf{g}) \tag{S3a}$$

$$\mathbf{u}_{AR}(\mathbf{k}) = \sum_{\mathbf{g}} e^{\imath\mathbf{k}\cdot\mathbf{g}}\mathbf{u}_{AR}(\mathbf{g}) \tag{S3b}$$

gives, after inserting them into Eq. (S2):

$$E^{(0)} = \frac{1}{\Omega}\sum_{\sigma}\Re\mathrm{Tr}\Bigg\{\int' d\mathbf{k}\left(\mathbf{v}(\mathbf{k})+\mathbf{u}_{AR}(\mathbf{k})+\mathbf{H}^{\sigma\sigma(0)}(\mathbf{k})\right) \times \mathbf{C}^{\sigma\sigma(0)}(\mathbf{k})\mathbf{f}_{\sigma}(\mathbf{k})\left[\mathbf{C}^{\sigma\sigma(0)}(\mathbf{k})\right]^{\dagger}\Bigg\} \tag{S4}$$

Then defining the matrix:

$$\Theta^{\sigma\sigma'}(\mathbf{k}) = \delta_{\sigma,\sigma'}\left[\mathbf{C}^{\sigma\sigma(0)}(\mathbf{k})\right]^{\dagger}\left(\mathbf{v}(\mathbf{k})+\mathbf{u}_{AR}(\mathbf{k})+\mathbf{H}^{\sigma\sigma(0)}(\mathbf{k})\right)\mathbf{C}^{\sigma\sigma(0)}(\mathbf{k}) \tag{S5}$$

And inserting Eq. (S5) into Eq. (S4) by exploiting the invariance of the trace to cyclic permutations gives:

$$E^{(0)} = \frac{1}{\Omega}\sum_{\sigma}\int' d\mathbf{k}\;\Re\mathrm{Tr}\left\{\mathbf{f}_{\sigma O}(\mathbf{k})\Theta^{\sigma\sigma}_{OO}(\mathbf{k})\right\} \tag{S6}$$

### B. First-Order Energy

From Eq. (39a) and using the fact that the zeroth-order Hamiltonian $\mathbf{H}^{(0)}(\mathbf{g})$ is pure-real, we find that all three terms in Eq. (S1c) involve the trace of a pure-real Hermitian matrix with a pure-imaginary Hermitian matrix. Therefore all three terms go to zero by Hermiticity:

$$E^{(1)} = 0 \tag{S7}$$

### C. Second-Order Energy

Proceeding as in Eq. (A6) of Paper 2, we may rewrite Eq. (S1d) as:

$$\begin{aligned} E^{(2)} &= \sum_{\sigma}\sum_{\mathbf{g}}\Re\mathrm{Tr}\left[\left(\mathbf{H}^{\sigma\sigma(0)}(\mathbf{g})\right)\mathbf{P}^{\sigma\sigma(2)}(\mathbf{g})\right] \\ &+ \frac{1}{2}\sum_{\sigma\sigma'}\sum_{\mathbf{g}}\Re\mathrm{Tr}\left[\left(\mathbf{F}^{\sigma\sigma'(1)}(\mathbf{g})\right)\mathbf{P}^{\sigma'\sigma(1)}(\mathbf{g})\right] \\ &+ \frac{1}{2}\sum_{\sigma\sigma'}\sum_{\mathbf{g}}\Re\mathrm{Tr}\left[\mathbf{u}_{SO}^{\sigma\sigma'}(\mathbf{g})\mathbf{P}^{\sigma'\sigma(1)}(\mathbf{g})\right] = T_1^{(2)}+T_2^{(2)}+T_3^{(2)} \end{aligned} \tag{S8}$$

We now turn to simplfying the first term $T_1^{(2)}$ in Eq. (S8). Writing the second-order density matrix using Eq. (C5), as well as the fact that the zeroth-order Hamiltonian $\mathbf{H}^{\sigma\sigma(0)}(\mathbf{g})$ is pure-real in direct-space gives:

$$\begin{aligned} T_1^{(2)} &= \frac{2}{\Omega}\sum_{\sigma}\sum_{\mathbf{g}}\Re\mathrm{Tr}\Bigg\{\int' d\mathbf{k}e^{\imath\mathbf{k}\cdot\mathbf{g}}\mathbf{H}^{\sigma\sigma(0)}(\mathbf{g}) \\ &\times \mathbf{C}^{\sigma\sigma(0)}(\mathbf{k})\Bigg(\mathbf{f}_{\sigma}(\mathbf{k})\left[\mathbf{U}^{\sigma\sigma\mathscr{R}(2)}(\mathbf{k})\right]^{\dagger}+\mathbf{U}^{\sigma\sigma\mathscr{R}(2)}(\mathbf{k})\mathbf{f}_{\sigma}(\mathbf{k}) \\ &+ \sum_{\sigma'}\mathbf{U}^{\sigma\sigma'\mathscr{R}(1)}(\mathbf{k})\mathbf{f}_{\sigma'}(\mathbf{k})\left[\mathbf{U}^{\sigma'\sigma\mathscr{R}(1)}(\mathbf{k})\right]^{\dagger}+\sum_{\sigma'}\mathbf{U}^{\sigma\sigma'\mathscr{I}(1)}(\mathbf{k})\mathbf{f}_{\sigma'}(\mathbf{k})\left[\mathbf{U}^{\sigma'\sigma\mathscr{I}(1)}(\mathbf{k})\right]^{\dagger}\Bigg)\left[\mathbf{C}^{\sigma\sigma(0)}(\mathbf{k})\right]^{\dagger}\Bigg\} \end{aligned} \tag{S9}$$

Then, using Eq. (31) and the invariance of the trace to cyclic permutations:

$$\begin{aligned} T_1^{(2)} &= \frac{2}{\Omega}\sum_{\sigma}\mathscr{R}\mathrm{Tr}\Bigg\{\int' d\mathbf{k}\;\left[\mathbf{C}^{\sigma\sigma(0)}(\mathbf{k})\right]^{\dagger}\mathbf{H}^{\sigma\sigma(0)}(\mathbf{k})\mathbf{C}^{\sigma\sigma(0)}(\mathbf{k}) \\ &\times \Bigg(\mathbf{f}_{\sigma}(\mathbf{k})\left[\mathbf{U}^{\sigma\sigma\mathscr{R}(2)}(\mathbf{k})\right]^{\dagger}+\mathbf{U}^{\sigma\sigma\mathscr{R}(2)}(\mathbf{k})\mathbf{f}_{\sigma}(\mathbf{k}) \\ &+ \sum_{\sigma'}\Bigg\{\mathbf{U}^{\sigma\sigma'\mathscr{R}(1)}(\mathbf{k})\mathbf{f}_{\sigma'}(\mathbf{k})\left[\mathbf{U}^{\sigma'\sigma\mathscr{R}(1)}(\mathbf{k})\right]^{\dagger}+\mathbf{U}^{\sigma\sigma'\mathscr{I}(1)}(\mathbf{k})\mathbf{f}_{\sigma'}(\mathbf{k})\left[\mathbf{U}^{\sigma'\sigma\mathscr{I}(1)}(\mathbf{k})\right]^{\dagger}\Bigg\}\Bigg)\Bigg\} \end{aligned} \tag{S10}$$

Now, the first line of Eq. (S10) is just the diagonal matrix of zeroth-order band-structure energies $\varepsilon^{\sigma(0)}(\mathbf{k}) = \left[\mathbf{C}^{\sigma\sigma(0)}(\mathbf{k})\right]^{\dagger}\mathbf{H}^{\sigma\sigma(0)}(\mathbf{k})\mathbf{C}^{\sigma\sigma(0)}(\mathbf{k})$ so that we obtain, by using also the Hermiticity of $\mathbf{U}_{OO}^{\sigma\sigma\mathscr{R}(2)}(\mathbf{k})$:

$$\begin{aligned} T_1^{(2)} &= \frac{2}{\Omega}\sum_{\sigma}\mathscr{R}\mathrm{Tr}\Bigg\{\int' d\mathbf{k}\, 2\varepsilon_O^{\sigma(0)}(\mathbf{k})\mathbf{f}_{\sigma O}(\mathbf{k})\mathbf{U}_{OO}^{\sigma\sigma\mathscr{R}(2)}(\mathbf{k}) \\ &+ \varepsilon_V^{\sigma(0)}(\mathbf{k})\sum_{\sigma'}\left(\mathbf{U}_{VO}^{\sigma\sigma'\mathscr{R}(1)}(\mathbf{k})\mathbf{f}_{\sigma' O}(\mathbf{k})\left[\mathbf{U}_{OV}^{\sigma'\sigma\mathscr{R}(1)}(\mathbf{k})\right]^{\dagger} + \mathbf{U}_{VO}^{\sigma\sigma'\mathscr{I}(1)}(\mathbf{k})\mathbf{f}_{\sigma' O}(\mathbf{k})\left[\mathbf{U}_{OV}^{\sigma'\sigma\mathscr{I}(1)}(\mathbf{k})\right]^{\dagger}\right)\Bigg\} \end{aligned} \tag{S11}$$

Finally, using Eq. (29a), we obtain:

$$\begin{aligned} T_1^{(2)} &= \frac{2}{\Omega}\sum_{\sigma\sigma'}\sum_{m}^{occ}\sum_{p}^{virt}\int' d\mathbf{k}\, f_{\sigma m}(\mathbf{k})\left(\varepsilon_p^{\sigma'(0)}(\mathbf{k}) - \varepsilon_m^{\sigma(0)}(\mathbf{k})\right) \\ &\times \Re\left\{\left[U_{pm}^{\sigma'\sigma\mathscr{R}(1)}(\mathbf{k})\right]^{*} U_{pm}^{\sigma'\sigma\mathscr{R}(1)}(\mathbf{k}) + \left[U_{pm}^{\sigma'\sigma\mathscr{I}(1)}(\mathbf{k})\right]^{*} U_{pm}^{\sigma'\sigma\mathscr{I}(1)}(\mathbf{k})\right\} \end{aligned} \tag{S12}$$

We now consider the second term $T_2^{(2)}$ in Eq. (S8), using Eqs. (37b) and (38), we obtain:

$$\begin{aligned} T_2^{(2)} &= \frac{1}{2\Omega}\sum_{\sigma\sigma'}\sum_{\mathbf{g}}\Re\mathrm{Tr}\Bigg\{\int d\mathbf{k}\, e^{\imath\mathbf{k}\cdot\mathbf{g}}\mathbf{H}^{\sigma\sigma'(1)}(\mathbf{g})\Bigg(\mathbf{C}^{\sigma'\sigma'(0)}(\mathbf{k})\mathbf{f}_{\sigma'}(\mathbf{k})\left[\mathbf{U}^{\sigma'\sigma(1)}(\mathbf{k})\right]^{\dagger}\left[\mathbf{C}^{\sigma\sigma(0)}(\mathbf{k})\right]^{\dagger} \\ &+ \mathbf{C}^{\sigma'\sigma'(0)}(\mathbf{k})\mathbf{U}^{\sigma'\sigma(1)}(\mathbf{k})\mathbf{f}_{\sigma}(\mathbf{k})\left[\mathbf{C}^{\sigma\sigma(0)}(\mathbf{k})\right]^{\dagger}\Bigg)\Bigg\} \end{aligned} \tag{S13}$$

where we note that the integral over $\mathbf{k}$ has no prime in Eq. (S13) because it runs over all points in the FBZ. Using Eq. (31) and the invariance of the trace to a cyclic permutation we get:

$$\begin{aligned} T_2^{(2)} &= \frac{1}{2\Omega}\sum_{\sigma\sigma'}\Re\mathrm{Tr}\Bigg\{\int d\mathbf{k}\,\left[\mathbf{C}^{\sigma\sigma(0)}(\mathbf{k})\right]^{\dagger}\mathbf{H}^{\sigma\sigma'(1)}(\mathbf{k})\mathbf{C}^{\sigma'\sigma'(0)}(\mathbf{k}) \\ &\times \left(\mathbf{f}_{\sigma'}(\mathbf{k})\left[\mathbf{U}^{\sigma'\sigma(1)}(\mathbf{k})\right]^{\dagger} + \mathbf{U}^{\sigma'\sigma(1)}(\mathbf{k})\mathbf{f}_{\sigma}(\mathbf{k})\right)\Bigg\} \end{aligned} \tag{S14}$$

Then, using Eqs. (23) as well as (26) and the Hermiticity of $\mathbf{G}_{OV}^{\sigma'\sigma(1)}(\mathbf{k})$ gives:

$$\begin{aligned} T_2^{(2)} &= \frac{1}{2\Omega}\sum_{\sigma\sigma'}\Re\mathrm{Tr}\Bigg\{\int d\mathbf{k}\,\Bigg(\mathbf{G}_{VO}^{\sigma\sigma'(1)}(\mathbf{k})\mathbf{f}_{\sigma' O}(\mathbf{k})\left[\mathbf{U}_{OV}^{\sigma'\sigma(1)}(\mathbf{k})\right]^{\dagger} \\ &+ \mathbf{G}_{OV}^{\sigma\sigma'(1)}(\mathbf{k})\mathbf{U}_{VO}^{\sigma'\sigma(1)}(\mathbf{k})\mathbf{f}_{\sigma O}(\mathbf{k})\Bigg)\Bigg\} \\ &= \frac{1}{\Omega}\sum_{\sigma\sigma'}\sum_{m}^{occ}\sum_{p}^{virt}\Re\left\{\int d\mathbf{k}\, f_{\sigma m}(\mathbf{k})G_{pm}^{\sigma'\sigma(1)}(\mathbf{k})\left[U_{pm}^{\sigma'\sigma(1)}(\mathbf{k})\right]^{*}\right\} \\ &= -\frac{1}{\Omega}\sum_{\sigma\sigma'}\sum_{m}^{occ}\sum_{p}^{virt}\int d\mathbf{k}\, f_{\sigma m}(\mathbf{k})\left(\varepsilon_p^{\sigma'(0)}(\mathbf{k}) - \varepsilon_m^{\sigma(0)}(\mathbf{k})\right) \\ &\times \Re\left\{\left[U_{pm}^{\sigma'\sigma(1)}(\mathbf{k})\right]^{*} U_{pm}^{\sigma'\sigma(1)}(\mathbf{k})\right\} \end{aligned} \tag{S15}$$

Finally, limiting the integral over $\mathbf{k}$ in Eq. (S15) to positive points and using Eqs. (32b), (C2), (35a) and (35b) gives:

$$\begin{aligned} T_2^{(2)} &= -\frac{2}{\Omega}\sum_{\sigma\sigma'}\sum_{m}^{occ}\sum_{p}^{virt}\int' d\mathbf{k}\, f_{\sigma m}(\mathbf{k})\left(\varepsilon_p^{\sigma'(0)}(\mathbf{k}) - \varepsilon_m^{\sigma(0)}(\mathbf{k})\right) \\ &\times \Re\left\{\left[U_{pm}^{\sigma'\sigma\mathscr{R}(1)}(\mathbf{k})\right]^{*} U_{pm}^{\sigma'\sigma\mathscr{R}(1)}(\mathbf{k}) + \left[U_{pm}^{\sigma'\sigma\mathscr{I}(1)}(\mathbf{k})\right]^{*} U_{pm}^{\sigma'\sigma\mathscr{I}(1)}(\mathbf{k})\right\} \end{aligned} \tag{S16}$$

Substituting Eqs. (S12) and (S16) for the terms $T_1^{(2)}$ and $T_2^{(2)}$ into Eq. (S8), we find that $T_1^{(2)}$ cancels with $T_2^{(2)}$, so we are left with the contribution from $T_3^{(2)}$:

$$E^{(2)} = \frac{1}{2}\sum_{\sigma\sigma'}\sum_{\mathbf{g}} \Re\mathrm{Tr}\left[\mathbf{u}_{SO}^{\sigma\sigma'}(\mathbf{g})\mathbf{P}^{\sigma'\sigma(1)}(\mathbf{g})\right] \tag{S17}$$

Eq. (S17) can be simplified by proceeding as in Eqs. (S13) and (S14) to get:

$$\begin{aligned} E^{(2)} &= \frac{1}{2\Omega}\sum_{\sigma\sigma'} \Re\mathrm{Tr}\left\{ \int d\mathbf{k}\, \left[\mathbf{C}^{\sigma\sigma(0)}(\mathbf{k})\right]^{\dagger} \mathbf{u}_{SO}^{\sigma\sigma'}(\mathbf{k})\mathbf{C}^{\sigma'\sigma'(0)}(\mathbf{k}) \right. \\ &\quad \left. \times \left(\mathbf{f}_{\sigma'}(\mathbf{k})\left[\mathbf{U}^{\sigma'\sigma(1)}(\mathbf{k})\right]^{\dagger} + \mathbf{U}^{\sigma'\sigma(1)}(\mathbf{k})\mathbf{f}_{\sigma}(\mathbf{k})\right)\right\} \end{aligned} \tag{S18}$$

Then, inserting the Hermitian matrix of SO integrals in the basis of crystalline orbitals $\Xi^{\sigma\sigma'}$ of Eq. (41) into Eq. (S18) gives:

$$E^{(2)} = \frac{1}{\Omega}\sum_{\sigma\sigma'} \Re\mathrm{Tr}\left\{ \int d\mathbf{k}\, \mathbf{f}_{\sigma O}(\mathbf{k})\Xi_{OV}^{\sigma\sigma'}(\mathbf{k})\mathbf{U}_{VO}^{\sigma'\sigma(1)}(\mathbf{k})\right\} \tag{S19}$$

Finally, limiting the integral over $\mathbf{k}$ in Eq. (S19) to points with positive coordinates and using Eqs. (35a), (35b), (41) and Eq. (C2) gives:

$$E^{(2)} = \frac{2}{\Omega}\sum_{\sigma\sigma'} \Re\mathrm{Tr}\left\{ \int' d\mathbf{k}\, \mathbf{f}_{\sigma O}(\mathbf{k}) \left(\Xi_{OV}^{\sigma\sigma'\mathscr{R}}(\mathbf{k})\mathbf{U}_{VO}^{\sigma'\sigma\mathscr{R}(1)}(\mathbf{k}) + \Xi_{OV}^{\sigma\sigma'\mathscr{I}}(\mathbf{k})\mathbf{U}_{VO}^{\sigma'\sigma\mathscr{I}(1)}(\mathbf{k})\right)\right\} \tag{S20}$$

which matches Eq. (42) of the main text

### D. Third-Order Energy

Proceeding as in Eqs. (A13)-(A17) of Paper 2 [1], we may rewrite Eq. (S1e) as:

$$\begin{aligned} E^{(3)} &= \sum_{\sigma}\sum_{\mathbf{g}} \Re\mathrm{Tr}\left[\mathbf{H}^{\sigma\sigma(0)}(\mathbf{g})\mathbf{P}^{\sigma\sigma(3)}(\mathbf{g})\right] \\ &+ \sum_{\sigma\sigma'}\sum_{\mathbf{g}} \Re\mathrm{Tr}\left[\mathbf{H}^{\sigma\sigma'(1)}(\mathbf{g})\mathbf{P}^{\sigma'\sigma(2)}(\mathbf{g})\right] \\ &= T_1^{(3)} + T_2^{(3)} \end{aligned} \tag{S21}$$

We consider the first term $T_1^{(3)}$ in Eq. (S21) this term can be simplified, by using the following equation for the third-order direct-space density matrix, obtained as a perturbation-theory expansion of Eqs. (36) and (38):

$$\begin{aligned} \mathbf{P}^{\sigma\sigma'(3)}(\mathbf{g}) &= \frac{1}{\Omega}\int d\mathbf{k}\, e^{\imath\mathbf{k}\cdot\mathbf{g}} \left[\mathbf{C}^{\sigma\sigma(0)}(\mathbf{k})\left\{\mathbf{f}_{\sigma}(\mathbf{k})\left[\mathbf{U}^{\sigma\sigma'(3)}(\mathbf{k})\right]^{\dagger} + \mathbf{U}^{\sigma\sigma'(3)}(\mathbf{k})\mathbf{f}_{\sigma'}(\mathbf{k})\right.\right. \\ &+ \left.\left.\sum_{\sigma''}\left(\mathbf{U}^{\sigma\sigma''(2)}(\mathbf{k})\mathbf{f}_{\sigma''}(\mathbf{k})\left[\mathbf{U}^{\sigma''\sigma'(1)}(\mathbf{k})\right]^{\dagger} + \mathbf{U}^{\sigma\sigma''(1)}(\mathbf{k})\mathbf{f}_{\sigma''}(\mathbf{k})\left[\mathbf{U}^{\sigma''\sigma'(2)}(\mathbf{k})\right]^{\dagger}\right)\right\}\left[\mathbf{C}^{\sigma'\sigma'(0)}(\mathbf{k})\right]^{\dagger}\right] \end{aligned} \tag{S22}$$

as well as the invariance of trace to a cyclic permutation, and proceeding as in Eqs. (S9)-(S11) to get:

$$\begin{aligned} T_1^{(3)} &= \frac{1}{\Omega}\sum_{\sigma} \Re\mathrm{Tr}\left\{ \int d\mathbf{k}\, \varepsilon^{\sigma(0)}(\mathbf{k})\left(\mathbf{f}_{\sigma}(\mathbf{k})\left[\mathbf{U}^{\sigma\sigma(3)}(\mathbf{k})\right]^{\dagger} + \mathbf{U}^{\sigma\sigma(3)}(\mathbf{k})\mathbf{f}_{\sigma}(\mathbf{k})\right.\right. \\ &+ \left.\left.\sum_{\sigma'}\left\{\mathbf{U}^{\sigma\sigma'(2)}(\mathbf{k})\mathbf{f}_{\sigma'}(\mathbf{k})\left[\mathbf{U}^{\sigma'\sigma(1)}(\mathbf{k})\right]^{\dagger} + \mathbf{U}^{\sigma\sigma'(1)}(\mathbf{k})\mathbf{f}_{\sigma'}(\mathbf{k})\left[\mathbf{U}^{\sigma'\sigma(2)}(\mathbf{k})\right]^{\dagger}\right\}\right)\right\} \end{aligned} \tag{S23}$$

Using the third-order orthogonality condition (see Eq. (31) of Paper 2 [1]) and the fact that the diagonal matrices $\mathbf{f}_\sigma(\mathbf{k})$ and $\varepsilon^{\sigma(0)}(\mathbf{k})$ commute, we obtain:

$$\begin{aligned} T_1^{(3)} &= \frac{1}{\Omega}\sum_\sigma \mathscr{R}\mathrm{Tr}\Bigg\{\int d\mathbf{k}\Bigg(-\varepsilon_O^{\sigma(0)}(\mathbf{k})\Bigg\{\sum_{\sigma'}\Big[\mathbf{U}_{OV}^{\sigma\sigma'(2)}(\mathbf{k})\Big]^\dagger \mathbf{U}_{VO}^{\sigma'\sigma(1)}(\mathbf{k}) \\ &+ \Big[\mathbf{U}_{OV}^{\sigma\sigma'(1)}(\mathbf{k})\Big]^\dagger \mathbf{U}_{VO}^{\sigma'\sigma(2)}(\mathbf{k})\Bigg\}\mathbf{f}_{\sigma O}(\mathbf{k}) + \varepsilon_V^{\sigma(0)}(\mathbf{k})\sum_{\sigma'}\Bigg\{\mathbf{U}_{VO}^{\sigma\sigma'(2)}(\mathbf{k})\mathbf{f}_{\sigma' O}(\mathbf{k})\Big[\mathbf{U}_{OV}^{\sigma'\sigma(1)}(\mathbf{k})\Big]^\dagger \\ &+ \mathbf{U}_{VO}^{\sigma\sigma'(1)}(\mathbf{k})\mathbf{f}_{\sigma' O}(\mathbf{k})\Big[\mathbf{U}_{OV}^{\sigma'\sigma(2)}(\mathbf{k})\Big]^\dagger\Bigg\}\Bigg)\Bigg\} \end{aligned} \tag{S24}$$

We now move on to simplifying the second term $T_2^{(3)}$ in Eq. (S21). Using Eqs. (22), (38) and (C4) we obtain:

$$\begin{aligned} T_2^{(3)} &= \frac{1}{\Omega}\sum_{\sigma\sigma'}\Re\mathrm{Tr}\Bigg\{\int d\mathbf{k}\,\mathbf{G}^{\sigma\sigma'(1)}(\mathbf{k})\Bigg(\mathbf{f}_{\sigma'}(\mathbf{k})\Big[\mathbf{U}^{\sigma'\sigma(2)}(\mathbf{k})\Big]^\dagger + \mathbf{U}^{\sigma'\sigma(2)}(\mathbf{k})\mathbf{f}_\sigma(\mathbf{k}) \\ &+ \sum_{\sigma''}\mathbf{U}^{\sigma'\sigma''(1)}(\mathbf{k})\mathbf{f}_{\sigma''}(\mathbf{k})\Big[\mathbf{U}^{\sigma''\sigma(1)}(\mathbf{k})\Big]^\dagger\Bigg)\Bigg\} \end{aligned} \tag{S25}$$

We now make use of the first-order perturbation equation, Eq. (20), to get:

$$\mathbf{G}^{\sigma\sigma'(1)}(\mathbf{k}) = \mathbf{U}^{\sigma\sigma'(1)}(\mathbf{k})\varepsilon^{\sigma'(0)}(\mathbf{k}) - \varepsilon^{\sigma(0)}(\mathbf{k})\mathbf{U}^{\sigma\sigma'(1)}(\mathbf{k}) + \varepsilon^{\sigma\sigma'(1)}(\mathbf{k}) \tag{S26}$$

Inserting Eq. (S26) into Eq. (S25) gives:

$$\begin{aligned} T_2^{(3)} &= \frac{1}{\Omega}\sum_{\sigma\sigma'}\Re\mathrm{Tr}\Bigg\{\int d\mathbf{k}\Bigg(\mathbf{U}^{\sigma\sigma'(1)}(\mathbf{k})\varepsilon^{\sigma'(0)}(\mathbf{k})\mathbf{f}_{\sigma'}(\mathbf{k})\Big[\mathbf{U}^{\sigma'\sigma(2)}(\mathbf{k})\Big]^\dagger \\ &- \varepsilon^{\sigma(0)}(\mathbf{k})\mathbf{U}^{\sigma\sigma'(1)}(\mathbf{k})\mathbf{f}_{\sigma'}(\mathbf{k})\Big[\mathbf{U}^{\sigma'\sigma(2)}(\mathbf{k})\Big]^\dagger + \varepsilon^{\sigma\sigma'(1)}(\mathbf{k})\mathbf{f}_{\sigma'}(\mathbf{k})\Big[\mathbf{U}^{\sigma'\sigma(2)}(\mathbf{k})\Big]^\dagger \\ &+ \mathbf{U}^{\sigma\sigma'(1)}(\mathbf{k})\varepsilon^{\sigma'(0)}(\mathbf{k})\mathbf{U}^{\sigma'\sigma(2)}(\mathbf{k})\mathbf{f}_\sigma(\mathbf{k}) - \varepsilon^{\sigma(0)}(\mathbf{k})\mathbf{U}^{\sigma\sigma'(1)}(\mathbf{k})\mathbf{U}^{\sigma'\sigma(2)}(\mathbf{k})\mathbf{f}_\sigma(\mathbf{k}) \\ &+ \varepsilon^{\sigma\sigma'(1)}(\mathbf{k})\mathbf{U}^{\sigma'\sigma(2)}(\mathbf{k})\mathbf{f}_\sigma(\mathbf{k}) + \mathbf{G}^{\sigma\sigma'(1)}(\mathbf{k})\sum_{\sigma''}\mathbf{U}^{\sigma'\sigma''(1)}(\mathbf{k})\mathbf{f}_{\sigma''}(\mathbf{k})\Big[\mathbf{U}^{\sigma''\sigma(1)}(\mathbf{k})\Big]^\dagger\Bigg)\Bigg\} \end{aligned} \tag{S27}$$

Now writing Eq. (S27) explicitly in terms of occ-virt blocks and using Eqs. (25) and (28):

$$\begin{aligned} T_2^{(3)} &= \frac{1}{\Omega}\sum_{\sigma\sigma'}\Re\mathrm{Tr}\Bigg\{\int d\mathbf{k}\Bigg(\mathbf{U}_{VO}^{\sigma\sigma'(1)}(\mathbf{k})\varepsilon_O^{\sigma'(0)}(\mathbf{k})\mathbf{f}_{\sigma' O}(\mathbf{k})\Big[\mathbf{U}_{OV}^{\sigma'\sigma(2)}(\mathbf{k})\Big]^\dagger \\ &- \varepsilon_V^{\sigma(0)}(\mathbf{k})\mathbf{U}_{VO}^{\sigma\sigma'(1)}(\mathbf{k})\mathbf{f}_{\sigma' O}(\mathbf{k})\Big[\mathbf{U}_{OV}^{\sigma'\sigma(2)}(\mathbf{k})\Big]^\dagger + \mathbf{G}_{OO}^{\sigma\sigma'(1)}(\mathbf{k})\mathbf{f}_{\sigma' O}(\mathbf{k})\Big[\mathbf{U}_{OO}^{\sigma'\sigma(2)}(\mathbf{k})\Big]^\dagger \\ &+ \mathbf{U}_{OV}^{\sigma\sigma'(1)}(\mathbf{k})\varepsilon_V^{\sigma'(0)}(\mathbf{k})\mathbf{U}_{VO}^{\sigma'\sigma(2)}(\mathbf{k})\mathbf{f}_{\sigma O}(\mathbf{k}) - \varepsilon_O^{\sigma(0)}(\mathbf{k})\mathbf{U}_{OV}^{\sigma\sigma'(1)}(\mathbf{k})\mathbf{U}_{VO}^{\sigma'\sigma(2)}(\mathbf{k})\mathbf{f}_{\sigma O}(\mathbf{k}) \\ &+ \mathbf{G}_{OO}^{\sigma\sigma'(1)}(\mathbf{k})\mathbf{U}_{OO}^{\sigma'\sigma(2)}(\mathbf{k})\mathbf{f}_{\sigma O}(\mathbf{k}) + \mathbf{G}_{VV}^{\sigma\sigma'(1)}(\mathbf{k})\sum_{\sigma''}\mathbf{U}_{VO}^{\sigma'\sigma''(1)}(\mathbf{k})\mathbf{f}_{\sigma'' O}(\mathbf{k})\Big[\mathbf{U}_{OV}^{\sigma''\sigma(1)}(\mathbf{k})\Big]^\dagger\Bigg)\Bigg\} \end{aligned} \tag{S28}$$

Substituting Eqs. (29a) and (29b) in Eq. (S28):

$$
\begin{aligned}
T_2^{(3)} &= \frac{1}{\Omega}\sum_{\sigma\sigma'}\Re\mathrm{Tr}\Bigg\{\int d\mathbf{k}\,\Bigg(\mathbf{U}_{VO}^{\sigma\sigma'(1)}(\mathbf{k})\varepsilon_{O}^{\sigma'(0)}(\mathbf{k})\mathbf{f}_{\sigma'O}(\mathbf{k})\left[\mathbf{U}_{OV}^{\sigma'\sigma(2)}(\mathbf{k})\right]^{\dagger}\\
&- \varepsilon_{V}^{\sigma(0)}(\mathbf{k})\mathbf{U}_{VO}^{\sigma\sigma'(1)}(\mathbf{k})\mathbf{f}_{\sigma'O}(\mathbf{k})\left[\mathbf{U}_{OV}^{\sigma'\sigma(2)}(\mathbf{k})\right]^{\dagger}\\
&- \frac{1}{2}\mathbf{G}_{OO}^{\sigma\sigma'(1)}(\mathbf{k})\mathbf{f}_{\sigma'O}(\mathbf{k})\left(\sum_{\sigma''}\left[\mathbf{U}_{OV}^{\sigma'\sigma''(1)}(\mathbf{k})\right]^{\dagger}\mathbf{U}_{VO}^{\sigma''\sigma(1)}(\mathbf{k})\right)\\
&+ \mathbf{U}_{OV}^{\sigma\sigma'(1)}(\mathbf{k})\varepsilon_{V}^{\sigma'(0)}(\mathbf{k})\mathbf{U}_{VO}^{\sigma'\sigma(2)}(\mathbf{k})\mathbf{f}_{\sigma O}(\mathbf{k}) - \varepsilon_{O}^{\sigma(0)}(\mathbf{k})\mathbf{U}_{OV}^{\sigma\sigma'(1)}(\mathbf{k})\mathbf{U}_{VO}^{\sigma'\sigma(2)}(\mathbf{k})\mathbf{f}_{\sigma O}(\mathbf{k})\\
&- \frac{1}{2}\mathbf{G}_{OO}^{\sigma\sigma'(1)}(\mathbf{k})\left(\sum_{\sigma''}\left[\mathbf{U}_{OV}^{\sigma'\sigma''(1)}(\mathbf{k})\right]^{\dagger}\mathbf{U}_{VO}^{\sigma''\sigma(1)}(\mathbf{k})\right)\mathbf{f}_{\sigma O}(\mathbf{k})\\
&+ \mathbf{G}_{VV}^{\sigma\sigma'(1)}(\mathbf{k})\sum_{\sigma''}\mathbf{U}_{VO}^{\sigma'\sigma''(1)}(\mathbf{k})\mathbf{f}_{\sigma''O}(\mathbf{k})\left[\mathbf{U}_{OV}^{\sigma''\sigma(1)}(\mathbf{k})\right]^{\dagger}\Bigg)\Bigg\}
\end{aligned}
\tag{S29}
$$

Taking the sum of Eqs. (S24) and (S29), terms one through four of Eq. (S24) cancel with terms 1, 5, 4, 2 of Eq. (S29), such that returning to Eq. (S21), we are left with an expression for the third order energy with terms 3, 6 and 7 of Eq. (S29):

$$
\begin{aligned}
E^{(3)} &= \frac{1}{\Omega}\sum_{\sigma\sigma'}\Re\mathrm{Tr}\Bigg\{\int d\mathbf{k}\,\Bigg(\mathbf{G}_{VV}^{\sigma\sigma'(1)}(\mathbf{k})\sum_{\sigma''}\mathbf{U}_{VO}^{\sigma'\sigma''(1)}(\mathbf{k})\mathbf{f}_{\sigma''O}(\mathbf{k})\left[\mathbf{U}_{OV}^{\sigma''\sigma(1)}(\mathbf{k})\right]^{\dagger}\\
&- \frac{1}{2}\left[\mathbf{f}_{\sigma O}(\mathbf{k})\mathbf{G}_{OO}^{\sigma\sigma'(1)}(\mathbf{k}) + \mathbf{G}_{OO}^{\sigma\sigma'(1)}(\mathbf{k})\mathbf{f}_{\sigma'O}(\mathbf{k})\right]\sum_{\sigma''}\left[\mathbf{U}_{OV}^{\sigma'\sigma''(1)}(\mathbf{k})\right]^{\dagger}\mathbf{U}_{VO}^{\sigma''\sigma(1)}(\mathbf{k})\Bigg)\Bigg\}
\end{aligned}
\tag{S30}
$$

Limiting the integral over $\mathbf{k}$ in Eq. (S30) to positive points in the FBZ:

$$
\begin{aligned}
E^{(3)} &= \frac{1}{\Omega}\sum_{\sigma\sigma'}\Re\mathrm{Tr}\Bigg\{\int' d\mathbf{k}\,\Bigg(\mathbf{G}_{VV}^{\sigma\sigma'(1)}(\mathbf{k})\sum_{\sigma''}\mathbf{U}_{VO}^{\sigma'\sigma''(1)}(\mathbf{k})\mathbf{f}_{\sigma''O}(\mathbf{k})\left[\mathbf{U}_{OV}^{\sigma''\sigma(1)}(\mathbf{k})\right]^{\dagger}\\
&+ \mathbf{G}_{VV}^{\sigma\sigma'(1)}(-\mathbf{k})\sum_{\sigma''}\mathbf{U}_{VO}^{\sigma'\sigma''(1)}(-\mathbf{k})\mathbf{f}_{\sigma''O}(-\mathbf{k})\left[\mathbf{U}_{OV}^{\sigma''\sigma(1)}(-\mathbf{k})\right]^{\dagger}\\
&- \frac{1}{2}\left[\mathbf{f}_{\sigma O}(\mathbf{k})\mathbf{G}_{OO}^{\sigma\sigma'(1)}(\mathbf{k}) + \mathbf{G}_{OO}^{\sigma\sigma'(1)}(\mathbf{k})\mathbf{f}_{\sigma'O}(\mathbf{k})\right]\sum_{\sigma''}\left[\mathbf{U}_{OV}^{\sigma'\sigma''(1)}(\mathbf{k})\right]^{\dagger}\mathbf{U}_{VO}^{\sigma''\sigma(1)}(\mathbf{k})\\
&- \frac{1}{2}\left[\mathbf{f}_{\sigma O}(-\mathbf{k})\mathbf{G}_{OO}^{\sigma\sigma'(1)}(-\mathbf{k}) + \mathbf{G}_{OO}^{\sigma\sigma'(1)}(-\mathbf{k})\mathbf{f}_{\sigma'O}(-\mathbf{k})\right]\sum_{\sigma''}\left[\mathbf{U}_{OV}^{\sigma'\sigma''(1)}(-\mathbf{k})\right]^{\dagger}\mathbf{U}_{VO}^{\sigma''\sigma(1)}(-\mathbf{k})\Bigg)\Bigg\}
\end{aligned}
\tag{S31}
$$

Then, inserting Eqs. (34a)-(35b) and Eq. (C2) into Eq. (S31) gives:

$$
\begin{aligned}
E^{(3)} \;=\; & \frac{2}{\Omega}\sum_{\sigma\sigma'}\Re\mathrm{Tr}\Bigg\{\int' d\mathbf{k}\,\Bigg(\mathbf{G}_{VV}^{\sigma\sigma'\mathscr{R}(1)}(\mathbf{k})\sum_{\sigma''}\mathbf{U}_{VO}^{\sigma'\sigma''\mathscr{R}(1)}(\mathbf{k})\mathbf{f}_{\sigma''O}(\mathbf{k})\left[\mathbf{U}_{OV}^{\sigma''\sigma\mathscr{R}(1)}(\mathbf{k})\right]^{\dagger} \\
& + \mathbf{G}_{VV}^{\sigma\sigma'\mathscr{R}(1)}(\mathbf{k})\sum_{\sigma''}\mathbf{U}_{VO}^{\sigma'\sigma''\mathscr{I}(1)}(\mathbf{k})\mathbf{f}_{\sigma''O}(\mathbf{k})\left[\mathbf{U}_{OV}^{\sigma''\sigma\mathscr{I}(1)}(\mathbf{k})\right]^{\dagger} \\
& + \mathbf{G}_{VV}^{\sigma\sigma'\mathscr{I}(1)}(\mathbf{k})\sum_{\sigma''}\mathbf{U}_{VO}^{\sigma'\sigma''\mathscr{R}(1)}(\mathbf{k})\mathbf{f}_{\sigma''O}(\mathbf{k})\left[\mathbf{U}_{OV}^{\sigma''\sigma\mathscr{I}(1)}(\mathbf{k})\right]^{\dagger} \\
& + \mathbf{G}_{VV}^{\sigma\sigma'\mathscr{I}(1)}(\mathbf{k})\sum_{\sigma''}\mathbf{U}_{VO}^{\sigma'\sigma''\mathscr{I}(1)}(\mathbf{k})\mathbf{f}_{\sigma''O}(\mathbf{k})\left[\mathbf{U}_{OV}^{\sigma''\sigma\mathscr{R}(1)}(\mathbf{k})\right]^{\dagger} \\
& - \frac{1}{2}\left[\mathbf{f}_{\sigma O}(\mathbf{k})\mathbf{G}_{OO}^{\sigma\sigma'\mathscr{R}(1)}(\mathbf{k})+\mathbf{G}_{OO}^{\sigma\sigma'\mathscr{R}(1)}(\mathbf{k})\mathbf{f}_{\sigma' O}(\mathbf{k})\right]\sum_{\sigma''}\left[\mathbf{U}_{OV}^{\sigma'\sigma''\mathscr{R}(1)}(\mathbf{k})\right]^{\dagger}\mathbf{U}_{VO}^{\sigma''\sigma\mathscr{R}(1)}(\mathbf{k}) \\
& - \frac{1}{2}\left[\mathbf{f}_{\sigma O}(\mathbf{k})\mathbf{G}_{OO}^{\sigma\sigma'\mathscr{R}(1)}(\mathbf{k})+\mathbf{G}_{OO}^{\sigma\sigma'\mathscr{R}(1)}(\mathbf{k})\mathbf{f}_{\sigma' O}(\mathbf{k})\right]\sum_{\sigma''}\left[\mathbf{U}_{OV}^{\sigma'\sigma''\mathscr{I}(1)}(\mathbf{k})\right]^{\dagger}\mathbf{U}_{VO}^{\sigma''\sigma\mathscr{I}(1)}(\mathbf{k}) \\
& - \frac{1}{2}\left[\mathbf{f}_{\sigma O}(\mathbf{k})\mathbf{G}_{OO}^{\sigma\sigma'\mathscr{I}(1)}(\mathbf{k})+\mathbf{G}_{OO}^{\sigma\sigma'\mathscr{I}(1)}(\mathbf{k})\mathbf{f}_{\sigma' O}(\mathbf{k})\right]\sum_{\sigma''}\left[\mathbf{U}_{OV}^{\sigma'\sigma''\mathscr{R}(1)}(\mathbf{k})\right]^{\dagger}\mathbf{U}_{VO}^{\sigma''\sigma\mathscr{I}(1)}(\mathbf{k}) \\
& - \frac{1}{2}\left[\mathbf{f}_{\sigma O}(\mathbf{k})\mathbf{G}_{OO}^{\sigma\sigma'\mathscr{I}(1)}(\mathbf{k})+\mathbf{G}_{OO}^{\sigma\sigma'\mathscr{I}(1)}(\mathbf{k})\mathbf{f}_{\sigma' O}(\mathbf{k})\right]\sum_{\sigma''}\left[\mathbf{U}_{OV}^{\sigma'\sigma''\mathscr{I}(1)}(\mathbf{k})\right]^{\dagger}\mathbf{U}_{VO}^{\sigma''\sigma\mathscr{R}(1)}(\mathbf{k})\Bigg)\Bigg\}
\end{aligned}
\tag{S32}
$$

which matches Eq. (43) of the main text.

## III. INPUT DECKS FOR CALCULATION ON THE W DICHALCOGENIDE LAYERS

### A. $WSe_2$ small-core

```
WSe2 SC
CRYSTAL
0 0 0
194
3.1532 12.323
2
274 0.333333333334 0.666666666667 0.25000
234 0.333333333334 0.666666666667 0.62250
SLABCUT
0 0 1
1 3
SYMMREMO
END
274 14
STUTSC
0 0 2 2. 1.
 15.000000000 -0.53984569304
 12.000000000 1.0228484726
0 0 1 2. 1.
 5.2610967725 1.0000000000
0 0 1 0. 1.
 0.92785370307 1.0000000000
0 0 1 0. 1.
 0.40334458241 1.0000000000
0 0 1 0. 1.
 0.15 1.0000000000
0 2 4 6. 1.
 7.2496570000 0.46749049338
```

```
 6.0848760000 -0.67718942302
 1.2523777812 0.53559619861
 0.58569208922 0.49083198365
0 2 1 0. 1.
 0.45 1.0000000000
0 2 1 0. 1.
 0.15 1.0000000000
0 3 1 4. 1.
 4.0131231332 1.0000000000
0 3 1 0. 1.
 1.6237452450 1.0000000000
0 3 1 0. 1.
 0.69187452392 1.0000000000
0 3 1 0. 1.
 0.27865835325 1.0000000000
0 4 1 0. 1.
 0.9 1.0
0 4 1 0. 1.
 0.3 1.0
234 9
STUTSC
0 0 8 2.0 1
2609.7204 0.001829
391.5228 0.009706
48.2893 0.071606
16.8019 -0.383980
3.5149 0.691926
1.5894 0.491893
0.3830 0.021091
0.1399 -0.003916
0 0 8 2.0 1
2609.7204 -0.000694
391.5228 -0.003866
48.2893 -0.024839
16.8019 0.140207
3.5149 -0.342280
1.5894 -0.364598
0.3830 0.698440
0.1399 0.532390
0 0 1 0.0 1
0.3830 1
0 0 1 0.0 1
0.1399 1
0 2 7 6.0 1
100.0192 0.004761
25.8909 -0.084899
6.2093 0.428655
2.6613 0.543060
1.0929 0.149283
0.3597 0.001071
0.1137 0.001019
0 2 7 4.0 1
100.0192 -0.001058
25.8909 0.021709
6.2093 -0.126243
2.6613 -0.193545
1.0929 0.047373
0.3597 0.591806
```

```
0.1137 0.499759
0 2 1 0.0 1
0.1137 1
0 3 7 10.0 1
128.508 0.011011
41.5212 0.077856
15.5182 0.232819
6.16082 0.401788
2.41134 0.408946
0.871936 0.168093
0.3656 0.007754
0 3 1 0.0 1
0.3656 1
99 0
END
TWOCOMPON
SOC
ENDTWO
DFT
XXLGRID
PBE0
ENDDFT
SHRINK
24 24
FMIXING
60
SMEAR
0.001
TOLINTEG
8 8 8 8 30
TOLDEE
8
MAXCYCLE
1000
END
```

### B. $WSe_2$ large-core

```
WSe2 LC
...      # same as WSe2 SC
234 8
STUTLC
0 0 3 2. 1
3.300301 0.385816
2.434170 -0.668512
0.713896 -0.384598
0 0 1 0. 1
0.528812 1.0
0 0 1 0. 1
0.211428 1.0
0 2 3 4. 1
5.153564 0.011117
2.057511 -0.102428
0.604512 0.226377
0 2 1 0. 1
0.291191 1.0
0 2 1 0. 1
```

```
0.133145 1.0
0 3 1 0. 1.
 0.9 1.0
0 3 1 0. 1.
 0.3 1.0
...      # same as WSe2 SC
```

### C. $WTe_2$ small-core

```
WTe2 SC
...      # same as WSe2 SC
252 9
STUTSC
0 0 8 2.0 1
2111.19 0.000612
311.691 0.003207
13.8226 0.405512
8.71748 -0.932588
1.98303 0.919657
0.970377 0.404671
0.279765 0.012366
0.106776 -0.001604
0 0 8 2.0 1
2111.19 0.000251
311.691 0.001457
13.8226 0.163702
8.71748 -0.398455
1.98303 0.578074
0.970377 0.327124
0.279765 -0.784654
0.106776 -0.499451
0 0 1 0.0 1
0.279765 1
0 0 1 0.0 1
0.106776 1
0 2 6 6.0 1
17.0629 0.089340
10.8306 -0.271168
2.59380 0.662023
1.12676 0.460744
0.300176 0.028809
0.097551 -0.003863
0 2 6 4.0 1
17.0629 -0.026861
10.8306 0.086304
2.59380 -0.273502
1.12676 -0.151390
0.300176 0.583976
0.097551 0.565014
0 2 1 0.0 1
0.097551 1
0 3 6 10.0 1
50.9106 0.003354
18.4647 -0.003642
4.27617 0.278080
1.89770 0.516348
0.786480 0.326571
```

```
0.2638 0.045152
0 3 1 0.0 1
0.2638 1
...      # same as WSe2 SC
```

### D. $WTe_2$ large-core

```
WTe2 LC
...      # same as WSe2 SC
252 8
STUTLC
0 0 3 2. 1
 4.620870 -0.076259
 3.407086 0.222163
 1.353795 -0.541514
0 0 1 0. 1
 0.278218 1.0
0 0 1 0. 1
 0.128403 1.0
0 2 3 4. 1
 4.772823 -0.038412
 3.508559 0.112992
 1.653984 -0.229605
0 2 1 0. 1
 0.326880 1.0
0 2 1 0. 1
 0.139746 1.0
0 3 1 0. 1.
 0.9 1.0
0 3 1 0. 1.
 0.3 1.0
...      # same as WSe2 SC
```

### E. $WPo_2$ small-core

```
WPo2 SC
...      # same as WSe2 SC
284 9
STUTSC
0 0 8 2.0 1
295.390 0.001383
21.2683 -0.105061
13.3379 0.591425
7.36521 -1.115697
1.78920 1.019162
0.884994 0.379879
0.285787 0.010781
0.109324 -0.001144
0 0 8 2.0 1
295.390 0.000683
21.2683 -0.038573
13.3379 0.251958
7.36521 -0.533016
1.78920 0.766901
0.884994 0.281878
0.285787 -0.839477
```

```
0.109324 -0.479272
0 0 1 0.0 1
0.285787 1
0 0 1 0.0 1
0.109324 1
0 2 6 6.0 1
11.5069 0.166364
7.72991 -0.427235
2.11894 0.696964
0.955323 0.471359
0.268352 0.029987
0.088494 -0.003487
0 2 6 4.0 1
11.5069 -0.055910
7.72991 0.151123
2.11894 -0.326160
0.955323 -0.161409
0.268352 0.601615
0.088494 0.555972
0 2 1 0.0 1
0.088494 1
0 3 6 10.0 1
18.7130 0.006694
7.05708 -0.067104
2.55062 0.325798
1.25069 0.495763
0.574256 0.293106
0.2330 0.054162
0 3 1 0.0 1
0.2330 1
...      # same as WSe2 SC
```

### F. $WPo_2$ large-core

```
WPo2 LC
...      # same as WSe2 SC
284 8
STUTLC
0 0 3 2. 1
2.549831 -0.093655
1.856210 0.874894
1.374970 -1.246453
0 0 1 0. 1
0.310166 1.0
0 0 1 0. 1
0.149667 1.0
0 2 3 4. 1
2.490870 -0.045917
1.843336 0.285716
1.365434 -0.407404
0 2 1 0. 1
0.296807 1.0
0 2 1 0. 1
0.128541 1.0
0 3 1 0. 1.
 0.9 1.0
0 3 1 0. 1.
```

```
 0.3 1.0
...      # same as WSe2 SC
```

### G. $WLv_2$ small-core

```
WLv2 SC
...      # same as WSe2 SC
316 26
STUTSH
0 0 1 2. 1
 78.0705  1.
0 0 1 2. 1
 55.7647  1.
0 0 1 0. 1
 39.8319  1.
0 0 1 0. 1
 28.4514   1.
0 0 1 0. 1
 20.3224   1.
0 0 1 0. 1
 6.9063    1.
0 0 1 0. 1
 1.6896    1.
0 0 1 0. 1
 0.7702    1.
0 0 1 0. 1
 0.3411    1.
0 0 1 0. 1
 0.1281    1.
0 2 1 6. 1
 14.7361   1.
0 2 1 4. 1
10.5258    1.
0 2 1 0. 1
 4.9125    1.
0 2 1 0. 1
 3.2831    1.
0 2 1 0. 1
 1.6303    1.
0 2 1 0. 1
 0.8507    1.
0 2 1 0. 1
 0.4122    1.
0 2 1 0. 1
 0.1960    1.
0 3 1 10. 1
 11.8693   1.
0 3 1 0. 1
 7.9083    1.
0 3 1 0. 1
 5.4441    1.
0 3 1 0. 1
 1.5987    1.
0 3 1 0. 1
 0.8199    1.
0 3 1 0. 1
 0.3978    1.
```

```
0 3 1 0. 1
 0.1728    1.
0 4 1 0. 1
 1.03259510 1.
...      # same as WSe2 SC
```

## IV. CONFIRMATION OF THE PT2′ APPROXIMATION ON SMALL MOLECULES

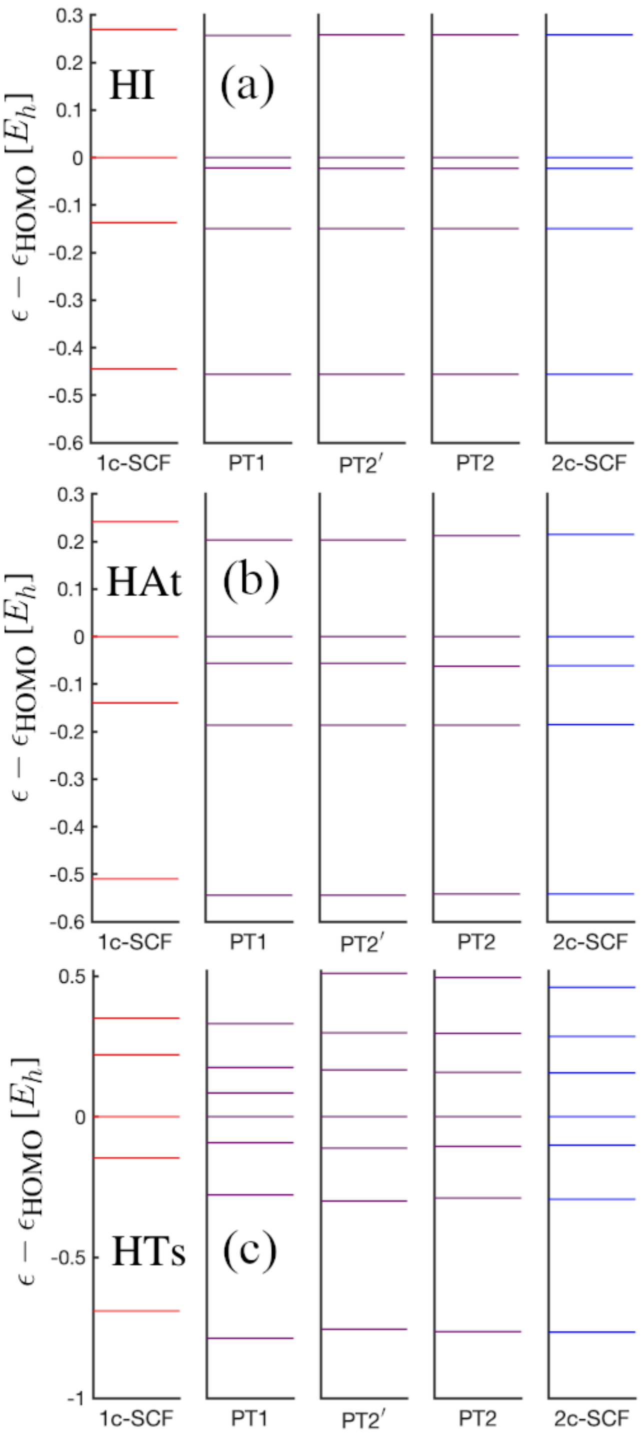


FIG. S1: KS eigenvalue spectrum calculated with the small-core RECPs and the PBE0 functional for the reported systems. See Ref. [1] for all computational details.

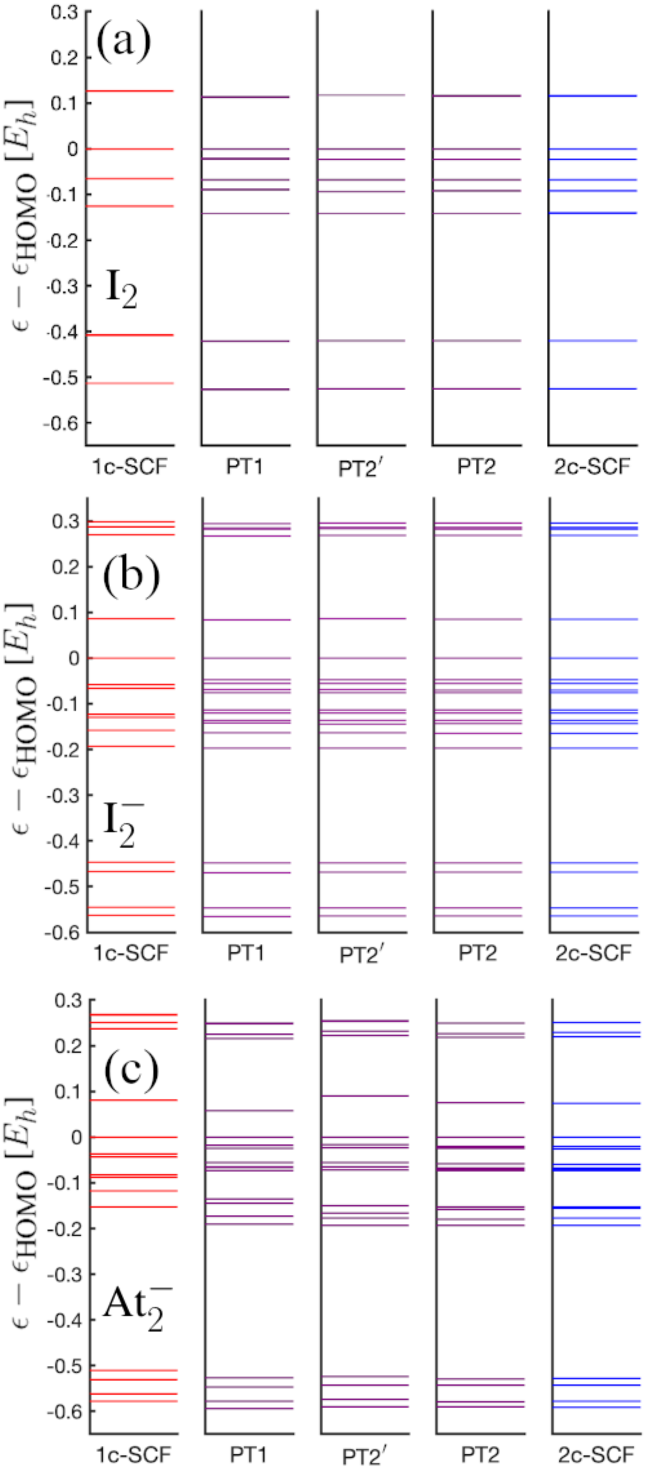


FIG. S2: KS eigenvalue spectrum calculated with the small-core RECPs and the PBE0 functional for the reported systems. See Ref. [1] for all computational details.

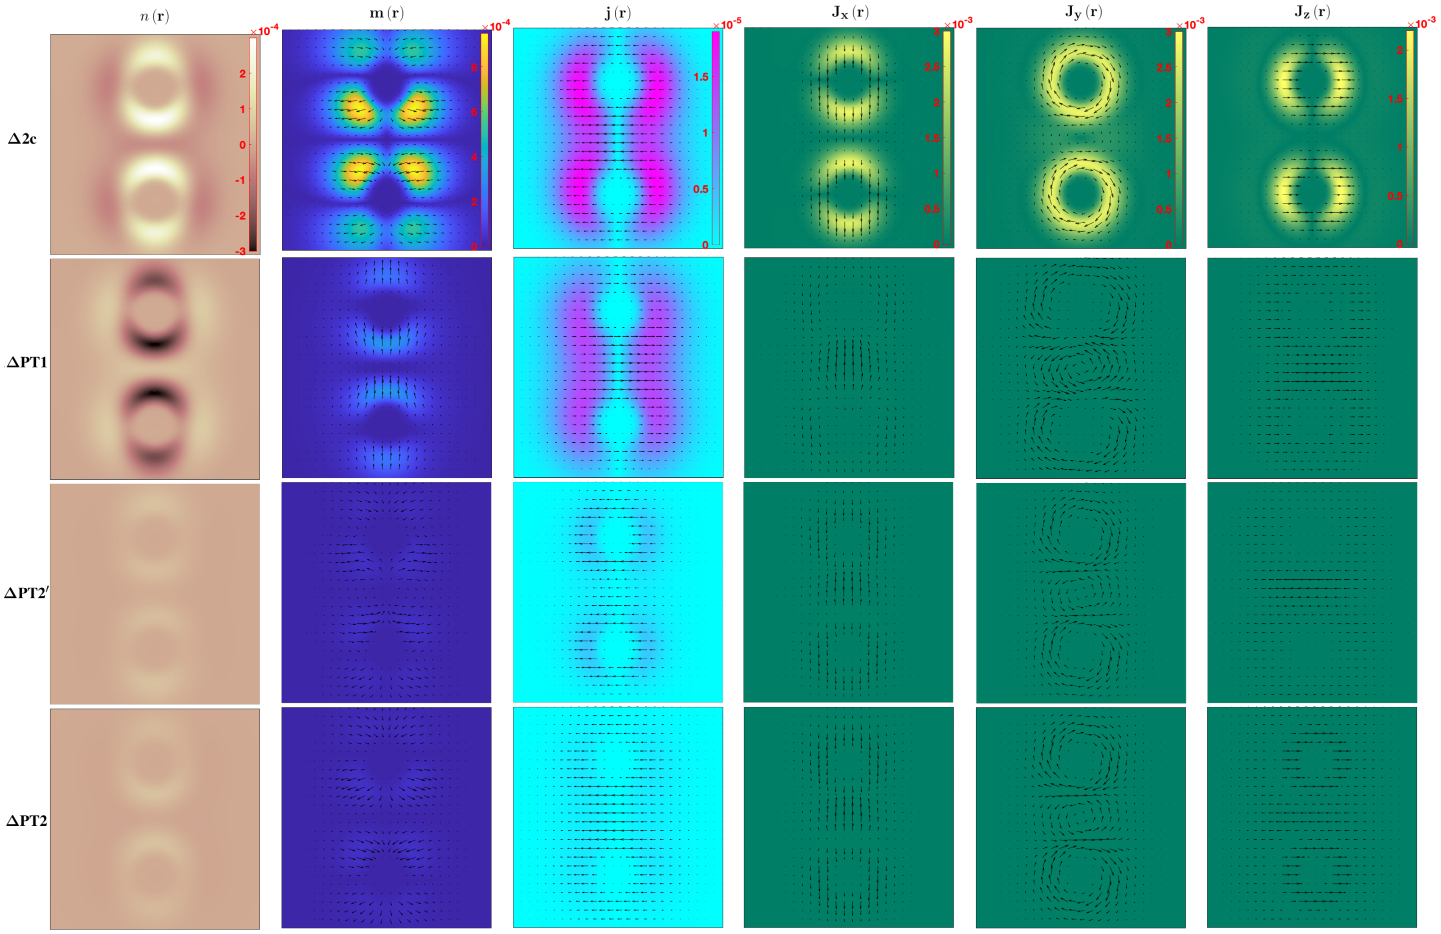


FIG. S3: Spatial distribution of differences of the SCDFT density variables for the system $I_2^-$ in the $xz$ plane, with the molecular axis along $z$, as obtained using the PBE0 functional and the small-core RECPs. The quantities in the first row are the differences $\Delta 2c = 2c - 1c$ where 2c denotes the distribution of the density variable calculated by 2c-SCF and 1c denotes a 1c-SCF calculation. Subsequent rows report $\Delta PT1 = PT1 - 2c$, $\Delta PT2 = PT2' - 2c$ and $\Delta PT2 = PT2 - 2c$, where PT1 (PT2′, PT2) denote the density variables obtained from a first- (second-)order perturbation theory treatment. From left to right the columns show the particle number density $n$, the magnetization $\mathbf{m}$, the orbital-current density $\mathbf{j}$ and the three spin-current densities $\mathbf{J}_x$, $\mathbf{J}_y$ and $\mathbf{J}_z$. When vector fields are plotted, the length and direction of the arrows represents the projection in the $xz$ plane. The color intensity represents the magnitude of the three dimensional vector. All quantities are plotted in atomic units.

## V. COMPLEMENT OF TABLE I FOR TOTAL ENERGIES

[1] J. K. Desmarais, A. Erba, J.-P. Flament, and B. Kirtman, J. Chem. Theor. Comput. **17**, 4712 (2021).

S1

TABLE S1: Total Energies (in $E_h$), with both large-core (LC) and small-core (SC) RECPs. The summed quantities $E^{\mathrm{PT2}} = E^{(0)} + E^{(2)}$ and $E^{\mathrm{PT3}} = E^{(0)} + E^{(2)} + E^{(3)}$ are also reported.

| | | $E^{(0)}$ | $E^{(2)}$ | $E^{(3)}$ | $E^{PT2}$ | $E^{PT3}$ | $E^{2c}$ |
|---|---|---|---|---|---|---|---|
| LC | $WSe_2$ | −86.388 | $-1.952\times10^{-2}$ | $5.102\times10^{-4}$ | −86.408 | −86.407 | −86.407 |
| | $WTe_2$ | −83.792 | $-2.490\times10^{-2}$ | $4.284\times10^{-4}$ | −83.817 | −83.816 | −83.816 |
| | $WPo_2$ | −83.463 | $-6.654\times10^{-2}$ | $-1.220\times10^{-3}$ | −83.529 | −83.530 | −83.531 |
| SC | $WSe_2$ | −813.948 | $-2.186\times10^{-2}$ | $5.566\times10^{-3}$ | −813.970 | −813.969 | −813.969 |
| | $WTe_2$ | −603.682 | $-3.731\times10^{-2}$ | $1.009\times10^{-3}$ | −603.719 | −603.718 | −603.718 |
| | $WPo_2$ | −543.232 | $-1.829\times10^{-1}$ | $9.053\times10^{-3}$ | −543.415 | −543.406 | −543.406 |
| | $WLv_2$ | −493.743 | $-3.243\times10^{0}$ | $-3.221\times10^{-1}$ | −496.987 | −497.309 | −497.247 |
